# Supplementary material for: Synthesizing Tasks for Block-based Programming
Source: arXiv:2006.16913 source file (2020-11-05)
Supplement: Supplementary file 1 [file 9.9_appendix_misc.tex]

% !TEX root =  main.tex
%%%%%%%%%%%%%%%%%%%%%%%%%%%%%%%%%%%%%%%%%%%%%%%%%%%%%%%%%%
%%%%%%%%%%%%%%%%%%%%%%%%%%%%%%%%%%%%%%%%%%%%%%%%%%%%%%%%%%
\section{Related Work}\label{appendix.relatedwork}
\paragraph{Related work. }
FIRST PARAGRAPH:
\begin{itemize}
\item Problem generation
\item Conceptual vs. procedural
\item Existing works on problem generation (other than coding) and differences
\end{itemize}

SECOND PARAGRAPH: Existing works on problem generation for coding and differences

THIRD PARAGRAPH: Existing works on visual content generation

FOURTH PARAGRAPH:
\begin{itemize}
\item Solution synthesizer, ITS hints, feedback
\item curriculum, teaching sequential tasks \cite{haug_teaching_2018}
\end{itemize}

%%%%%%%%%%%%%%%%%%%%%%%%%%%%%%%%%%%%%%%%%%%%%%%%%%%%%%%%%%
%%%%%%%%%%%%%%%%%%%%%%%%%%%%%%%%%%%%%%%%%%%%%%%%%%%%%%%%%%
%%%%%%%%%%%%%%%%%%%%%%%%%%%%%%%%%%%%%%%%%%%%%%%%%%%%%%%%%%
%%%%%%%%%%%%%%%%%%%%%%%%%%%%%%%%%%%%%%%%%%%%%%%%%%%%%%%%%%
\section{Misc}\label{appendix.misc}

%%%%%%%%%%%%%%%%%%%%%%%%%%%%%%%%%%%%%
\begin{figure}[t!]
	\centering
	%%%%%%%%%%%%%%%%%
	\begin{minipage}{0.50\textwidth}
			\begin{subfigure}[b]{1.0\textwidth}
				\centering
				{
					\begin{boxcode2col}{1.2cm}{6.2cm}{0.75}{1.0}
						\DSLCode \code &:= \textcode{def }\DSLRun() \DSLdo y \\
						\DSLRule \DSLRuleVar &:= \DSLStmtVar | \DSLRepeatForever  | \DSLStmtVar;\DSLRepeatForever \\
						% %
						\DSLRule \DSLStmtVar \hspace{1mm} &:= \DSLActionVar \text{ } | $\text{\DSLStmtVar};\text{\DSLStmtVar}$ | \DSLIf(\DSLBoolVar) \DSLdo $\text{\DSLStmtVar}$ | \DSLIf(\DSLBoolVar) \DSLdo $\text{\DSLStmtVar}$ \DSLElse $\text{\DSLStmtVar}$\\
						& \quad | \DSLWhile(\DSLBoolVar) \DSLdo  $\text{\DSLStmtVar}$  | \DSLRepeat(\DSLIterVar) \DSLdo $\text{\DSLStmtVar}$ \\
						\DSLRule \DSLRepeatForever &:= \DSLRepeatUntil(\DSLBoolGoal) \DSLdo $\text{\DSLStmtVar}$\\
						%  %
						\DSLAction \DSLActionVar &:= \DSLMove| \DSLTurnL | \DSLTurnR|  \DSLPutM | \DSLPickM \\
						%   %
						\DSLBool \DSLBoolVar &:= \DSLBoolPathA | \DSLBoolNoPathA | \DSLBoolPathL | \DSLBoolNoPathL \\
						& \quad | \DSLBoolPathR | \DSLBoolNoPathR  | \DSLBoolMarker  | \DSLBoolNoMarker \\
						%    %
						\DSLIter \DSLIterVar &:= $2$ | $3$ | $4$ | $5$ | $6$ | $7$ | $8$ | $9$ | $10$\\
						%\vspace{2mm}
					\end{boxcode2col}
					\vspace{-3mm}
					\caption{Code DSL}
					\vspace{0.5mm}
					\label{fig:mutation.1}
				}
			\end{subfigure}
		\\
		%%%%%%%%%%%%%%%%%
			\begin{subfigure}[b]{1.0\textwidth}
			\centering
			{
				\begin{boxcode}{9.0cm}{0.75}{1.0}
					\textbf{Input}: code \code, sketch \SDSLSketchVar $\leftarrow$ $\codetosketch(\code)$, parameters $\sketchparams(.| \code)$, $\delta_\text{thresh}$, $\delta_{r}$
					\\
					Note: \actionseq~is a sequence of actions: $\text{\SDSLAction}_{1}$, \ldots $\text{\SDSLAction}_{N}$
					\begin{enumerate}%[\ensuremath{\Delta_{1}}]
						\item[(\ensuremath{\Delta_{0}})] Constraint on generated code size based on $\code_{\textnormal{size}} \pm \delta_\text{thresh}$ 
						
						\item[(\ensuremath{\Delta_{1}})] For each $\text{\actionseq} \in \text{\SDSLSketchVar}$, constraints ensuring minimality of \actionseq 
						
						\item[(\ensuremath{\Delta_{2}})] Constraints induced on \actionseq~nested inside conditional \SDSLBool
						
						\item[(\ensuremath{\Delta_{3}})] Constraints induced by repeat: \{\text{\actionseq}\textsubscript{before};  \DSLRepeat\{\actionseq\} \text{\actionseq}\textsubscript{after}\}
						\begin{enumerate}[\leftmargin=0em]
							\item[i.] \actionseq~is not a suffix of \actionseq\textsubscript{before}
							\item[ii.] \actionseq~is not a prefix of \actionseq\textsubscript{after}
						\end{enumerate}
						
						\item[(\ensuremath{\Delta_{4}})]  For each \SDSLIter~$ \in \text{\SDSLSketchVar}: |\text{\SDSLIter} - \sketchparams(\text{\SDSLIter}| \code)| \leq \delta_{r}$
						
						\item[(\ensuremath{\Delta_{5}})]  For each \SDSLBool~$\in \text{\SDSLSketchVar}:$
						
						\begin{enumerate}[\leftmargin=0em]
							\item[i.] \sketchparams(\text{\SDSLBool}| \code)
							$\in$ \{ \DSLBoolPathA, \DSLBoolNoPathA \}
							$\Rightarrow$ \SDSLBool $\in$ \{ \DSLBoolPathA,\DSLBoolNoPathA \}
							
							\item[ii.] \sketchparams(\text{\SDSLBool}| \code) $\in$ \{ \DSLBoolPathL, \DSLBoolNoPathL 
							\text{\DSLBoolPathR }, \DSLBoolNoPathR \} 
							\item[] 
							$\Rightarrow$ \SDSLBool $\in$ \{ \DSLBoolPathL, \DSLBoolNoPathL, \DSLBoolPathR, \DSLBoolNoPathR \}
							
							\item[iii.] \sketchparams(\text{\SDSLBool}| \code) $\in$ \{\DSLBoolMarker, \DSLBoolNoMarker\} 
							\item[] $\Rightarrow$ \SDSLBool $\in$ \{ \DSLBoolMarker,\DSLBoolNoMarker\}
							
						\end{enumerate}
						
						\item[(\ensuremath{\Delta_{6}})] $\text{For each }\text{\actionseq} \in \text{\SDSLSketchVar}$, \localblockcons(\actionseq, $\sketchparams(\actionseq| \code)$). 
						\item[] \quad Only one block has actions added to them at a time.
						
						\vspace{-0.8em}
					\end{enumerate}
				\end{boxcode}
				\vspace{5mm}
				\caption{Sketch Constraint Types}
				\label{fig:mutation.3}
			}
		\end{subfigure}

	\end{minipage}
	\hspace{0.5em}
	%%%%%%%%%%%%%%%%%
	\begin{minipage}{0.40\textwidth}
	\begin{subfigure}[b]{1.0\textwidth}
					\centering
					{
						\begin{boxcode2col}{1.2cm}{6.2cm}{0.75}{1.0}
							\SDSLSketch \SDSLSketchVar  &:= \textcode{def }\DSLRun() \DSLdo $\text{\SDSLVarY}$ \\
							% %
						\DSLRule \SDSLVarY & := \SDSLSStmtVar | \SDSLVarG | \SDSLSStmtVar; \SDSLVarG \\
							% %
							\DSLRule \SDSLSStmtVar &:= \SDSLBlockVar | \SDSLSStmtVar;\SDSLSStmtVar |
							\DSLIf(\SDSLBool) \DSLdo $\text{\SDSLSStmtVar}$
							\\
							& \quad | \DSLIf(\SDSLBool) \DSLdo $\text{\SDSLSStmtVar}$ \DSLElse
							$\text{\SDSLSStmtVar}$ \\
						& \quad | \DSLWhile(\SDSLBool) \DSLdo $\text{\SDSLSStmtVar}$  | \DSLRepeat(\SDSLIter) \DSLdo $\text{\SDSLSStmtVar}$ \\
						% %
							\DSLRule \SDSLVarG & := \DSLRepeatUntil(\DSLBoolGoal) \DSLdo $\text{\SDSLSStmtVar}$ \\
						% %
							\DSLRule\SDSLBlockVar &:= $\phi$ |   \SDSLAction | \SDSLAction; \SDSLBlockVar\\
							%\vspace{2mm}
						\end{boxcode2col}
						\vspace{-3mm}
						\caption{Sketch DSL}
						%\vspace{0.5mm}
						\label{fig:mutation.2}
					}
		\end{subfigure}    	
	%%%%%%%%%%%%%%%%%
	\\
	\begin{subfigure}[b]{0.52\textwidth}
		\centering
		{
			\begin{boxcode}{3.8cm}{0.60}{0.65}
				\textcode{def }\DSLRun\textcode{()\{}\\
				\quad \DSLRepeatUntil\textcode{(}\DSLBoolGoal\textcode{)\{}\\
				\quad \quad \DSLMove\\
				\quad \quad \DSLIf\textcode{(}\DSLBoolPathLeft\textcode{)\{}\\
				\quad \quad \quad \DSLTurnLeft\\
				\quad \quad \textcode{\}}\\
				\quad \textcode{\}}\\
				\textcode{\}}
				\\
				\\
			\vspace{-1.5mm}
			\end{boxcode}
			\vspace{-3mm}
			\caption{Solution code \code\textsuperscript{in}}
			\label{fig:mutation.4}
		}
	\end{subfigure}
	\begin{subfigure}[b]{.40\textwidth}
		\centering
		{
			
			\begin{boxcode}{3.8cm}{0.65}{0.45}
				\textcode{def }\DSLRun\textcode{()\{}\\
				{\small
				\quad
				$\text{\SDSLAction}^{1}_{1}$, $\text{\SDSLAction}^{2}_{1}$ \textcolor{blue}{(\actionseqb\textsubscript{1})}
				}
				\\
				\quad
				\DSLRepeatUntil\textcode{(}\DSLBoolGoal\textcode{)\{}\\
				{\small
				\quad \quad  
				$\text{\SDSLAction}^{1}_{2}$, $\text{\SDSLAction}^{2}_{2}$, $\text{\SDSLAction}^{3}_{2}$, 
				$\text{\SDSLAction}^{4}_{2}$, 
				$\text{\SDSLAction}^{5}_{2}$ \textcolor{blue}{(\actionseqb\textsubscript{2})}
				}
				\\
				
				\quad \quad \DSLIf\textcode{(}$\text{\SDSLBool}_{1}$\textcode{)\{}\\
				{\small
					\quad \quad  \quad
					$\text{\SDSLAction}^{1}_{3}$, $\text{\SDSLAction}^{2}_{3}$, $\text{\SDSLAction}^{3}_{3}$, 
					$\text{\SDSLAction}^{4}_{3}$, 
					$\text{\SDSLAction}^{5}_{3}$ \textcolor{blue}{(\actionseqb\textsubscript{2})}
				}
				\\
				\quad \quad \textcode{\}}\\
				\quad \textcode{\}}\\
				\textcode{\}}
				\\
				\vspace{-1.5mm}
			\end{boxcode}
			\vspace{-3mm}
			\caption{Sketch \textcode{Q}\textsuperscript{in}}
			\label{fig:mutation.5}
		}
	\end{subfigure}
	\\
	\begin{subfigure}[b]{1.0\textwidth}
		\centering
		{
			\begin{boxcode}{8.2cm}{0.75}{1.0}
				\textbf{Input}: \code\textsuperscript{in}, $\text{\textcode{Q}}^\text{in}$, \sketchparams($.| \text{\code}^\text{in}$) = ($\phi$ , $\text{\DSLMove}$,  $\text{\DSLTurnL}$, \DSLBoolPathL), \\
				\qquad \quad $\delta_\text{thresh} = 2$
				\begin{enumerate}
					\item[(\ensuremath{\Delta_1})] $\text{\actionseq}_{1}$, $\actionseq_{2}$, $\actionseq_{3}$ is minimal
					
					\item[(\ensuremath{\Delta_2})] $\text{\actionseq}_{3}$ in \DSLBool $\text{\SDSLBool}_{1} = \text{\DSLBoolPathL}$
					\begin{itemize}
						\item[] $\exists \text{\SDSLAction}_{3i} \in \{ \text{\SDSLAction}_{31}, \ldots , \text{\SDSLAction}_{35}\}$ s.t ($\text{\SDSLAction}_{3i} = $ \DSLTurnL
						
						\item[] $\land \text{ } \forall \text{\SDSLAction}_{3j} \in \{ \text{\SDSLAction}_{31}, \ldots , \text{\SDSLAction}_{3i} \}$ $\text{\SDSLAction}_{3j}$ $\notin$ \{\DSLMove, \DSLTurnR \})
					\end{itemize}
					
					\item[(\ensuremath{\Delta_2})] $\text{\actionseq}_{3}$ in \DSLBool $\text{\SDSLBool}_{1} = \text{\DSLBoolPathR}$
					
					\begin{itemize}
						\item[]$\exists \text{\SDSLAction}_{3i} \in \{ \text{\SDSLAction}_{31}, \ldots , \text{\SDSLAction}_{35}\}$ s.t ($\text{\SDSLAction}_{3i} = $ \DSLTurnR
						\item[] $\land \text{ } \forall \text{\SDSLAction}_{3j} \in \{ \text{\SDSLAction}_{31}, \ldots , \text{\SDSLAction}_{3i} \}$ $\text{\SDSLAction}_{3j} \notin $ \{\DSLMove, \DSLTurnL \})
					\end{itemize}
					
					\item[(\ensuremath{\Delta_5})] $\text{\SDSLBool}_{1}$ = \DSLBoolPathL $\lor$ $\text{\SDSLBool}_{1}$ = \DSLBoolPathR
					
					\item[(\ensuremath{\Delta_6})] $\localblockcons(\actionseq_{1}, \sketchparams(\actionseq_{1}| \code^\text{in}))$, 
					$\localblockcons(\actionseq_{2}, 
					\sketchparams(\actionseq_{2}| \code^\text{in}))$, 
					\item []  \qquad $\localblockcons(\actionseq_{3}, \sketchparams(\actionseq_{3}| \code^\text{in}))$
					\item[]
					\quad \quad Only one of $\actionseq_{1}, \actionseq_{2}, \actionseq_{3}$ have actions added to them.
					
					\vspace{-2mm}
				\end{enumerate}
				
			\end{boxcode}
			\vspace{-3mm}
			\caption{Sketch \SDSLSketchVar-Constraints}
			\label{fig:mutation.6}
		}
	\end{subfigure}	
	\end{minipage}
	%%%%%%%%%%%%%%%%%
	\caption{Illustration of Program Mutation}
	\label{fig:mutation}
\end{figure}

\clearpage

%%%%%%%%%%%%%%%%%%%%%%%%%%%%%%%%%%%%%
\begin{figure}[t!]
\centering
	%%%%%%%%%%%%%%%%%
\begin{minipage}{0.48\textwidth}
    \begin{minipage}{1.0\textwidth}
    \hspace{-4em}
	\begin{subfigure}[b]{1.0\textwidth}
	\centering
	{
	    \begin{boxcode2col}{1.2cm}{6.2cm}{0.75}{1.0}
		      \DSLCode \code &:= \textcode{def }\DSLRun() \DSLdo y \\
		      \DSLRule \DSLRuleVar &:= \DSLStmtVar | \DSLRepeatForever  | \DSLStmtVar;\DSLRepeatForever \\
		      % %
		      \DSLRule \DSLStmtVar \hspace{1mm} &:= \DSLActionVar \text{ } | $\text{\DSLStmtVar};\text{\DSLStmtVar}$ | \DSLIf(\DSLBoolVar) \DSLdo $\text{\DSLStmtVar}$ | \DSLIf(\DSLBoolVar) \DSLdo $\text{\DSLStmtVar}$ \DSLElse $\text{\DSLStmtVar}$\\
		      & \quad | \DSLWhile(\DSLBoolVar) \DSLdo  $\text{\DSLStmtVar}$  | \DSLRepeat(\DSLIterVar) \DSLdo $\text{\DSLStmtVar}$ \\
		      \DSLRule \DSLRepeatForever &:= \DSLRepeatUntil(\DSLBoolGoal) \DSLdo $\text{\DSLStmtVar}$\\
		      %  %
		      \DSLAction \DSLActionVar &:= \DSLMove| \DSLTurnL | \DSLTurnR|  \DSLPutM | \DSLPickM \\
		      %   %
		      \DSLBool \DSLBoolVar &:= \DSLBoolPathA | \DSLBoolNoPathA | \DSLBoolPathL | \DSLBoolNoPathL \\
		      & \quad | \DSLBoolPathR | \DSLBoolNoPathR  | \DSLBoolMarker  | \DSLBoolNoMarker \\
             %    %
		      \DSLIter \DSLIterVar &:= $2$ | $3$ | $4$ | $5$ | $6$ | $7$ | $8$ | $9$ | $10$\\
		      %\vspace{2mm}
		\end{boxcode2col}
		\vspace{-3mm}
		\caption{Code DSL}
		\vspace{0.5mm}
		\label{fig:mutation.1}
    }
    \end{subfigure}
    \end{minipage}
    \\
	%%%%%%%%%%%%%%%%%
	\begin{minipage}{1.0\textwidth}
	\hspace{-4em}
	\begin{subfigure}[b]{1.0\textwidth}
	\centering
	{
	    \begin{boxcode2col}{1.2cm}{6.2cm}{0.75}{1.0}
		      \SDSLSketch \SDSLSketchVar  &:= \textcode{def }\DSLRun() \DSLdo $\text{\SDSLVarY}$ \\
		      % %
		      \DSLRule \SDSLVarY & := \SDSLSStmtVar | \SDSLVarG | \SDSLSStmtVar; \SDSLVarG \\
		      % %
		      \DSLRule \SDSLSStmtVar &:= \SDSLBlockVar | \SDSLSStmtVar;\SDSLSStmtVar |
		     \DSLIf(\SDSLBool) \DSLdo $\text{\SDSLSStmtVar}$
		     \\
		     & \quad | \DSLIf(\SDSLBool) \DSLdo $\text{\SDSLSStmtVar}$ \DSLElse
		       $\text{\SDSLSStmtVar}$ \\
		       & \quad | \DSLWhile(\SDSLBool) \DSLdo $\text{\SDSLSStmtVar}$  | \DSLRepeat(\SDSLIter) \DSLdo $\text{\SDSLSStmtVar}$ \\
		       % %
		    \DSLRule \SDSLVarG & := \DSLRepeatUntil(\DSLBoolGoal) \DSLdo $\text{\SDSLSStmtVar}$ \\
		    % %
		     \DSLRule\SDSLBlockVar &:= $\phi$ |   \SDSLAction | \SDSLAction; \SDSLBlockVar\\
		      %\vspace{2mm}
		\end{boxcode2col}
		\vspace{-3mm}
		\caption{Sketch DSL}
		\vspace{0.5mm}
		\label{fig:mutation.2}
    }
    \end{subfigure}    
    \end{minipage}
\end{minipage}
	%%%%%%%%%%%%%%%%%
	\hspace{-5em}
	\begin{minipage}{0.48\textwidth}
	\begin{subfigure}[b]{1.0\textwidth}
	\centering
	{
		 \begin{boxcode}{9.0cm}{0.75}{1.0}
		 \textbf{Input}: code \code, sketch \SDSLSketchVar $\leftarrow$ $\codetosketch(\code)$, parameters $\sketchparams(.| \code)$, $\delta_\text{thresh}$, $\delta_{r}$
		 \\
		 Note: \actionseq~is a sequence of actions: $\text{\SDSLAction}_{1}$, \ldots $\text{\SDSLAction}_{N}$
    		 \begin{enumerate}%[\ensuremath{\Delta_{1}}]
    		     \item[(\ensuremath{\Delta_{0}})] Constraint on generated code size based on $\code_{\textnormal{size}} \pm \delta_\text{thresh}$ 
    		     
    		     \item[(\ensuremath{\Delta_{1}})] For each $\text{\actionseq} \in \text{\SDSLSketchVar}$, constraints ensuring minimality of \actionseq 
    		     
    		     \item[(\ensuremath{\Delta_{2}})] Constraints induced on \actionseq~nested inside conditional \SDSLBool
    		     
    		     \item[(\ensuremath{\Delta_{3}})] Constraints induced by repeat: \{\text{\actionseq}\textsubscript{before};  \DSLRepeat\{\actionseq\} \text{\actionseq}\textsubscript{after}\}
    		        \begin{enumerate}[\leftmargin=0em]
    		            \item[i.] \actionseq~is not a suffix of \actionseq\textsubscript{before}
    		            \item[ii.] \actionseq~is not a prefix of \actionseq\textsubscript{after}
    		        \end{enumerate}
    		        
    		 \item[(\ensuremath{\Delta_{4}})]  For each \SDSLIter~$ \in \text{\SDSLSketchVar}: |\text{\SDSLIter} - \sketchparams(\text{\SDSLIter}| \code)| \leq \delta_{r}$
    		
    		 \item[(\ensuremath{\Delta_{5}})]  For each \SDSLBool~$\in \text{\SDSLSketchVar}:$
    		 
    		 \begin{enumerate}[\leftmargin=0em]
    		     \item[i.] \sketchparams(\text{\SDSLBool}| \code)
		         $\in$ \{ \DSLBoolPathA, \DSLBoolNoPathA \}
		         $\Rightarrow$ \SDSLBool $\in$ \{ \DSLBoolPathA,\DSLBoolNoPathA \}
		        
		         \item[ii.] \sketchparams(\text{\SDSLBool}| \code) $\in$ \{ \DSLBoolPathL, \DSLBoolNoPathL 
		 \text{\DSLBoolPathR }, \DSLBoolNoPathR \} 
		\item[] 
		 $\Rightarrow$ \SDSLBool $\in$ \{ \DSLBoolPathL, \DSLBoolNoPathL, \DSLBoolPathR, \DSLBoolNoPathR \}
		 
		  \item[iii.] \sketchparams(\text{\SDSLBool}| \code) $\in$ \{\DSLBoolMarker, \DSLBoolNoMarker\} 
		  \item[] $\Rightarrow$ \SDSLBool $\in$ \{ \DSLBoolMarker,\DSLBoolNoMarker\}
		 
		 \end{enumerate}
		 
		 \item[(\ensuremath{\Delta_{6}})] $\text{For each }\text{\actionseq} \in \text{\SDSLSketchVar}$, \localblockcons(\actionseq, $\sketchparams(\actionseq| \code)$). 
		 \item[] \quad Only one block has actions added to them at a time.

		  \vspace{-0.8em}
    \end{enumerate}
		\end{boxcode}
		\vspace{-3mm}
		\caption{Sketch Constraint Types}
		\label{fig:mutation.3}
	}
    \end{subfigure}
    \end{minipage}
	%%%%%%%%%%%%%%%%%
		\begin{subfigure}[b]{.22\textwidth}
		\centering
		{
			\begin{boxcode}{3.8cm}{0.75}{0.7}
				\textcode{def }\DSLRun\textcode{()\{}\\
				\quad \DSLRepeatUntil\textcode{(}\DSLBoolGoal\textcode{)\{}\\
				\quad \quad \DSLMove\\
				\quad \quad \DSLIf\textcode{(}\DSLBoolPathLeft\textcode{)\{}\\
				\quad \quad \quad \DSLTurnLeft\\
				\quad \quad \textcode{\}}\\
				\quad \textcode{\}}\\
				\textcode{\}}
				\\
				\\
			\end{boxcode}
			\vspace{-2mm}
			\caption{Solution code \code\textsuperscript{in}}
			\label{fig:mutation.4}
		}
	\end{subfigure}
\begin{subfigure}[b]{.22\textwidth}
		\centering
		{
			
			\begin{boxcode}{3.8cm}{0.72}{0.65}
				\textcode{def }\DSLRun\textcode{()\{}\\
				{\small
					\quad
					$\text{\SDSLAction}^{1}_{1}$, $\text{\SDSLAction}^{2}_{1}$ \textcolor{blue}{(\actionseqb\textsubscript{1})}
				}
				\\
				\quad
				\DSLRepeatUntil\textcode{(}\DSLBoolGoal\textcode{)\{}\\
				{\small
					\quad \quad  
					$\text{\SDSLAction}^{1}_{2}$, $\text{\SDSLAction}^{2}_{2}$, $\text{\SDSLAction}^{3}_{2}$, 
					$\text{\SDSLAction}^{4}_{2}$, 
					$\text{\SDSLAction}^{5}_{2}$ \textcolor{blue}{(\actionseqb\textsubscript{2})}
				}
				\\
				
				\quad \quad \DSLIf\textcode{(}$\text{\SDSLBool}_{1}$\textcode{)\{}\\
				{\small
					\quad \quad  \quad
					$\text{\SDSLAction}^{1}_{3}$, $\text{\SDSLAction}^{2}_{3}$, $\text{\SDSLAction}^{3}_{3}$, 
					$\text{\SDSLAction}^{4}_{3}$, 
					$\text{\SDSLAction}^{5}_{3}$ \textcolor{blue}{(\actionseqb\textsubscript{2})}
				}
				\\
				\quad \quad \textcode{\}}\\
				\quad \textcode{\}}\\
				\textcode{\}}
				\\
			\end{boxcode}
			\vspace{-2mm}
			\caption{Sketch \textcode{Q}\textsuperscript{in}}
			\label{fig:mutation.5}
		}
	\end{subfigure}
    % \qquad
    % \quad
    % \quad
  % \hspace{0.3em}
	\begin{subfigure}[b]{0.50\textwidth}
	\centering
    {
    \begin{boxcode}{8.8cm}{0.75}{1.0}
    \textbf{Input}: \code\textsuperscript{in}, $\text{\textcode{Q}}^\text{in}$, \sketchparams($.| \text{\code}^\text{in}$) = ($\phi$ , $\text{\DSLMove}$,  $\text{\DSLTurnL}$, \DSLBoolPathL), \\
    \qquad \quad $\delta_\text{thresh} = 2$
        \begin{enumerate}
            \item[(\ensuremath{\Delta_1})] $\text{\actionseq}_{1}$, $\actionseq_{2}$, $\actionseq_{3}$ is minimal
            
            \item[(\ensuremath{\Delta_2})] $\text{\actionseq}_{3}$ in \DSLBool $\text{\SDSLBool}_{1} = \text{\DSLBoolPathL}$
            \begin{itemize}
             \item[] $\exists \text{\SDSLAction}_{3i} \in \{ \text{\SDSLAction}_{31}, \ldots , \text{\SDSLAction}_{35}\}$ s.t ($\text{\SDSLAction}_{3i} = $ \DSLTurnL
             
             \item[] $\land \text{ } \forall \text{\SDSLAction}_{3j} \in \{ \text{\SDSLAction}_{31}, \ldots , \text{\SDSLAction}_{3i} \}$ $\text{\SDSLAction}_{3j}$ $\notin$ \{\DSLMove, \DSLTurnR \})
            \end{itemize}
            
            \item[(\ensuremath{\Delta_2})] $\text{\actionseq}_{3}$ in \DSLBool $\text{\SDSLBool}_{1} = \text{\DSLBoolPathR}$
            
            \begin{itemize}
                \item[]$\exists \text{\SDSLAction}_{3i} \in \{ \text{\SDSLAction}_{31}, \ldots , \text{\SDSLAction}_{35}\}$ s.t ($\text{\SDSLAction}_{3i} = $ \DSLTurnR
                \item[] $\land \text{ } \forall \text{\SDSLAction}_{3j} \in \{ \text{\SDSLAction}_{31}, \ldots , \text{\SDSLAction}_{3i} \}$ $\text{\SDSLAction}_{3j} \notin $ \{\DSLMove, \DSLTurnL \})
            \end{itemize}
        
        \item[(\ensuremath{\Delta_5})] $\text{\SDSLBool}_{1}$ = \DSLBoolPathL $\lor$ $\text{\SDSLBool}_{1}$ = \DSLBoolPathR
        
        \item[(\ensuremath{\Delta_6})] $\localblockcons(\actionseq_{1}, \sketchparams(\actionseq_{1}| \code^\text{in}))$, 
        $\localblockcons(\actionseq_{2}, 
        \sketchparams(\actionseq_{2}| \code^\text{in}))$, 
        \item []  \qquad $\localblockcons(\actionseq_{3}, \sketchparams(\actionseq_{3}| \code^\text{in}))$
        \item[]
        \quad \quad Only one of $\actionseq_{1}, \actionseq_{2}, \actionseq_{3}$ have actions added to them.
        
         \vspace{-2mm}
        \end{enumerate}
   
	\end{boxcode}
		\vspace{-3mm}
		\caption{Sketch \SDSLSketchVar-Constraints}
		\label{fig:mutation.6}
	}
	\end{subfigure}
	\caption{Illustration of Program Mutation}
	\label{fig:mutation}
\end{figure}
%%%%%%%%%%%%%%%%%%%%%%%%%%%%%%%%%%%%%
